# Supplementary material for: Benchmarking Scientific Image Forgery Detectors
Source: arXiv:2105.12872 source file (2021-05-26)
Supplement: Supplementary file 1 [file suppl.tex]

%\REVIEW{We need to insert the tables in the supplementary material, so someone can use them to copy this results on their work.}

% Please add the following required packages to your document preamble:
% \usepackage{graphicx}
% Please add the following required packages to your document preamble:
% \usepackage{graphicx}

% Please add the following required packages to your document preamble:
% \usepackage{multirow}
% \usepackage{graphicx}

This section presents all scores (organized in tables) resulting from our evaluation; thus, one can easily compare a future solution with this baseline. In addition, we present output samples from all methods to each evaluated modality.
\subsection{\textit{Evaluation I}: Simple Forgery Figures}
Table \ref{tab:simple-f1} shows the evaluation of Simple Figure Forgery Detection with $\mbox{F1-score}_{TP}$ (indicated by the columns TP) and $\mbox{F1-score}_{CTP}$ (indicated by the columns CTP), both normalized in $[0,100]$.
Table \ref{tab:simple-p} shows the evaluation of Simple Figure Forgery Detection using Precision with true positive (TP) and consistent true positive (\textit{CTP}), both normalized in $[0,100]$.
Figure \ref{fig:sample-simple-forgery} presents output detection samples for all method applied to the evaluated Simple forgeries modalities. This figure includes $\mbox{F1-score}_{CTP}$ of the each detected map next to each method's name in the figure.

\subsection{\textit{Evaluation II}: Compound Forgery Figures}
Tables \ref{tab:compund-f1-l1}, \ref{tab:compund-f1-l2}, \ref{tab:compund-f1-l1} show the evaluation of Compound Figure Forgery Detection ranging the level of indicative letter verbosity from one to three using $\mbox{F1-score}_{TP}$ and $\mbox{F1-score}_{CTP}$ ; while Tables \ref{tab:compund-p-l1}, \ref{tab:compund-p-l2}, \ref{tab:compund-p-l1} show the same evaluation using  $\mbox{Precision}_{TP}$ and $\mbox{Precision}_{CTP}$. All tables scores are normalized in $[0,100]$.
Figure \ref{fig:sample-intra-forgery} presents output detection samples for all method applied to the evaluated Intra-Panel forgeries modalities, while Figure \ref{fig:sample-inter-forgery} applied to Inter-Panel forgeries modalities.

\begin{table}[]

\caption{Evaluation of Simple Figure Forgery Detection with F1-Score}
\centering
\resizebox{\textwidth}{!}{%
\begin{tabular}{|c|S|S|S|S|S|S|S|S|S|S|}
\hline
\multirow{3}{*}{\textbf{Modality}} & \multicolumn{10}{c|}{\textbf{Methods (F1-Score)}} \\ \cline{2-11} 
 & \multicolumn{2}{c|}{ZERNIKE-PM} & \multicolumn{2}{c|}{SIFT-PM} & \multicolumn{2}{c|}{SURF-VOLE} & \multicolumn{2}{c|}{SIFT-VOLE} & \multicolumn{2}{c|}{BUSTERNET} \\ \cline{2-11} 
 & TP & CTP  & TP &  CTP &  TP &  CTP & TP & CTP  & TP &  CTP  \\ \hline
Cleaning (Brute-Force) & \num{0.00} & \num{0.00} & \num{0.94} & \num{0.10} & \num{0.00} & \num{0.00} & \num{0.00} & \num{0.00} & \textbf{\num{3.55}} & \textbf{\num{2.59}} \\ \hline
Copy-Move (Flip) & \num{0.00} & \num{0.00} & \num{0.85} & \num{0.48} & \num{0.60} & \num{0.47} & \num{0.64} & \num{0.43} & \textbf{\num{1.95}} & \textbf{\num{1.19}} \\ \hline
Copy-Move (Random) & \num{8.90} &\num{8.63} & \num{13.47} & \num{11.13} & \num{3.03} & \num{3.01} & \num{4.67} & \num{4.61} & \textbf{\num{16.83}} & \textbf{\num{16.04}} \\ \hline
Copy-Move (Rotation) & \num{0.00} & \num{0.00} & \num{0.74} & \num{0.34} & \num{0.26} & \num{0.25} & \num{0.46} & \num{0.36} & \textbf{\num{5.19}} & \textbf{\num{2.42}} \\ \hline
Copy-move (Translation) & \num{1.14} &\num{0.96} & \num{4.98} & \num{3.38} & \num{0.25} & \num{0.25} & \num{0.55} & \num{0.50} & \textbf{\num{9.72}} & \textbf{\num{6.86}} \\ \hline
\textbf{Average} & \num{2.01} & \num{1.92} & \num{4.20} & \num{3.09} & \num{0.83} & \num{0.80} & \num{1.26} & \num{1.18} & \textbf{\num{7.45}} & \textbf{\num{5.82}} \\ \hline
%\multicolumn{4}{l}{\small *All scores are in $[0,100]$} \\
\end{tabular}%
\label{tab:simple-f1}
}
\end{table}
% Please add the following required packages to your document preamble:
% \usepackage{multirow}
% \usepackage{graphicx}
\begin{table*}[]

\caption{Evaluation of Simple Figure Forgery Detection with Precision}
\centering
\resizebox{\textwidth}{!}{%
%\begin{tabular}{|c|c|c|c|c|c|c|c|c|c|c|}
\begin{tabular}{|c|S|S|S|S|S|S|S|S|S|S|}
\hline
\multirow{3}{*}{\textbf{\textbf{Modality}}} & \multicolumn{10}{c|}{\textbf{Methods (Precision)}} \\ \cline{2-11} 
 & \multicolumn{2}{c|}{ZERNIKE-PM} & \multicolumn{2}{c|}{SIFT-PM} & \multicolumn{2}{c|}{SURF-VOLE} & \multicolumn{2}{c|}{SIFT-VOLE} & \multicolumn{2}{c|}{BUSTERNET} \\ \cline{2-11} 
 & TP  & CTP  & TP  & CTP  & TP  & CTP  & TP  & CTP  & TP  & CTP  \\ \hline
Cleaning (Brute-Force) & \num{0.00} & \num{0.00} & \num{1.06} & \num{0.12} & \num{0.00} & \num{0.00} & \num{0.00} & \num{0.00} & \textbf{\num{15.83}} & \textbf{\num{8.71}} \\ \hline
Copy-Move (Flip) & \num{0.00} & \num{0.00} & \num{1.13} & \num{0.67} & \num{0.96} & \num{0.77} & \num{1.04} & \num{0.75} & \textbf{\num{17.28}} & \textbf{\num{5.94}} \\ \hline
Copy-Move (Random) & \num{12.33} & \num{12.03} & \num{14.55} & \num{12.24} & \num{5.63} & \num{5.62} & \num{10.24} & \num{10.19} & \textbf{\num{58.61}} & \textbf{\num{46.56}} \\ \hline
Copy-Move (Rotation) & \num{0.00} & \num{0.00} & \num{0.82} & \num{0.36} & \num{0.34} & \num{0.33} & \num{0.68} & \num{0.60} & \textbf{\num{19.50}} & \textbf{\num{6.92}} \\ \hline
Copy-move (Translation) & \num{2.18} & \num{1.92} & \num{5.36} & \num{3.73} & \num{0.38} & \num{0.38} & \num{0.73} & \num{0.69} & \textbf{\num{29.14}} & \textbf{\num{17.12}} \\ \hline
\textbf{Average} & \num{2.90} & \num{2.79} & \num{4.59} & \num{3.43} & \num{1.46} & \num{1.42} & \num{2.54} & \num{2.45} & \textbf{\num{28.07}} & \textbf{\num{17.05}} \\ \hline
\end{tabular}%
\label{tab:simple-p}
}
\end{table*}

% Please add the following required packages to your document preamble:
% \usepackage{multirow}
% \usepackage{graphicx}
\begin{table*}[]
\caption{Evaluation of Compound Figure Detection on Level 1 of Verbosity with F1-Score}
\centering
\resizebox{\textwidth}{!}{%
%\begin{tabular}{|c|c|c|c|c|c|c|c|c|c|c|c|}
\begin{tabular}{|c|c|S|S|S|S|S|S|S|S|S|S|}
\hline
\multicolumn{2}{|c|}{\multirow{3}{*}{\textbf{Modality}}} & \multicolumn{10}{c|}{\textbf{Methods (F1-Score - Verbosity Level 1)}} \\ \cline{3-12} 
\multicolumn{2}{|c|}{} & \multicolumn{2}{c|}{ZERNIKE-PM} & \multicolumn{2}{c|}{SIFT-PM} & \multicolumn{2}{c|}{SURF-VOLE} & \multicolumn{2}{c|}{SIFT-VOLE} & \multicolumn{2}{c|}{BUSTERNET} \\ \cline{3-12} 
\multicolumn{2}{|c|}{} & TP  & CTP  & TP  & CTP  & TP  & CTP  & TP  & CTP  &  TP  &  CTP  \\ \hline
\multirow{9}{*}{\begin{tabular}[c]{@{}c@{}}Inter-Panel\\ Forgery\end{tabular}} & Copy-Move (Flip) & \num{0.18} & \num{0.04} & \num{6.52} & \num{4.88} & \num{3.86} & \num{3.35} & \num{3.91} & \num{3.74} & \textbf{\num{17.31}} & \textbf{\num{13.12}} \\ \cline{2-12} 
 & Copy-Move (Flip + Rotation 90°) & \num{0.94} & \num{0.85} & \num{1.82} & \num{0.70} & \num{0.56} & \num{0.54} & \num{1.30} & \num{1.26} & \textbf{\num{13.69}} & \textbf{\num{11.57}} \\ \cline{2-12} 
 & Copy-Move (None) & \num{6.81} & \num{6.65} & \num{58.45} & \num{55.76} & \num{57.12} & \num{56.85} & \textbf{\num{59.23}} & \textbf{\num{59.22}} & \num{18.39} & \num{14.26} \\ \cline{2-12} 
 & Copy-Move (Rotation 180°) & \num{0.08} & \num{0.00} & \num{3.86} & \num{1.38} & \textbf{\num{66.77}} & \textbf{\num{66.47}} & \num{57.80} & \num{57.80} & \num{16.03} & \num{13.11} \\ \cline{2-12} 
 & Copy-Move (Rotation 90°) & \num{0.02} & \num{0.00} &\num{ 1.}71 & \num{0.42} & \num{33.94} & \num{33.91} & \textbf{\num{42.56}} & \textbf{\num{42.56}} & \num{15.09} & \num{12.35} \\ \cline{2-12} 
 & Copy-Move (Retouching) & \num{51.32} & \textbf{\num{51.03}} & \textbf{\num{52.86}} & \num{50.02} & \num{40.76} & \num{40.75} & \num{37.45} & \num{37.45} & \num{16.41} & \num{13.08} \\ \cline{2-12} 
 & Splicing & \num{1.60} & \num{1.47} & \num{1.98} & \num{1.59} & \textbf{\num{2.11}} & \textbf{\num{1.93}} & \num{0.54} & \num{0.47} & \num{1.30} & \num{1.07} \\ \cline{2-12} 
 & Overlap & \num{0.00} & \num{0.00} & \num{0.27} & \num{0.12} & \num{3.09} & \num{3.00} & \num{6.45} & \textbf{\num{6.23}} & \textbf{\num{8.15}} & \num{5.44} \\ \cline{2-12} 
 & \textbf{Average} & \num{7.62} & \num{7.50} & \num{15.93} & \num{14.36} & \num{26.03} & \num{25.85} & \textbf{\num{26.16}} & \textbf{\num{26.09}} & \num{13.30} & \num{10.50} \\ \hline \hline
\multirow{6}{*}{\begin{tabular}[c]{@{}c@{}}Intra-Panel\\ Forgery\end{tabular}} & Cleaning (Brute-Force) & \num{0.06} & \num{0.03} & \num{0.23} &\num{0.08} & \num{0.00} & \num{0.00} & \num{0.00} & \num{0.00} & \textbf{\num{1.30}} & \textbf{\num{1.07}} \\ \cline{2-12} 
 & Copy-Move (Flip) & \num{0.00} & \num{0.00} & \num{0.18} & \num{0.08} & \num{0.01} & \num{0.01} & \num{0.00} & \num{0.00} & \textbf{\num{1.31}} & \textbf{\num{1.06}} \\ \cline{2-12} 
 & Copy-Move (Random) & \textbf{\num{2.57}} & \textbf{\num{2.44}} & \num{2.39} & \num{1.79} & \num{2.42} & \num{2.29} & \num{1.16} & \num{1.10} & \num{1.46} & \num{1.19} \\ \cline{2-12} 
 & Copy-Move (Rotation) & \num{0.00} & \num{0.00} & \num{0.08} & \num{0.02} & \num{0.18} & \num{0.13} & \num{0.03} & \num{0.02} & \textbf{\num{1.17}} & \textbf{\num{0.92}} \\ \cline{2-12} 
 & Copy-move (Translation) & \num{0.99} & \num{0.91} & \textbf{\num{1.19}} & \textbf{\num{0.80}} & \num{0.68} & \num{0.51} & \num{0.17} & \num{0.15} & \num{0.80} & \num{0.67} \\ \cline{2-12} 
 & \textbf{Average} & \num{0.72} & \num{0.68} & \num{0.81} & \num{0.56} & \num{0.66} & \num{0.59} & \num{0.27} & \num{0.25} & \textbf{\num{1.21}} & \textbf{\num{0.98}} \\ \hline
\end{tabular}%
\label{tab:compund-f1-l1}
}
\end{table*}

% Please add the following required packages to your document preamble:
% \usepackage{multirow}
% \usepackage{graphicx}
\begin{table*}[]
\caption{Evaluation of Compound Figure Detection on Level 2 of Verbosity with F1-Score}
\centering
\resizebox{\textwidth}{!}{%
\begin{tabular}{|c|c|c|c|c|c|c|c|c|c|c|c|}
\hline
\multicolumn{2}{|c|}{\multirow{3}{*}{\textbf{Modality}}} & \multicolumn{10}{c|}{\textbf{Methods (F1-Score - Verbosity Level 2)}} \\ \cline{3-12} 
\multicolumn{2}{|c|}{} & \multicolumn{2}{c|}{ZERNIKE-PM} & \multicolumn{2}{c|}{SIFT-PM} & \multicolumn{2}{c|}{SURF-VOLE} & \multicolumn{2}{c|}{SIFT-VOLE} & \multicolumn{2}{c|}{BUSTERNET} \\ \cline{3-12} 
\multicolumn{2}{|c|}{} &  TP  &  CTP  &  TP  &  CTP  &  TP  &  CTP  &  TP  &  CTP  &  TP  &  CTP  \\ \hline
\multirow{9}{*}{\begin{tabular}[c]{@{}c@{}}Inter-Panel\\ Forgery\end{tabular}} & Copy-Move (Flip) & \num{0.19} & \num{0.05} & \num{6.23} & \num{4.60} & \num{3.46} & \num{2.61} & \num{1.77} & \num{1.24} & \textbf{\num{17.29}} & \textbf{\num{13.31}} \\ \cline{2-12} 
 & Copy-Move (Flip + Rotation 90°) & \num{0.95} & \num{0.88} & \num{1.81} & \num{0.58} & \num{0.69} & \num{0.47} & \num{1.54} & \num{0.74} & \textbf{\num{13.66}} & \textbf{\num{11.23}} \\ \cline{2-12} 
 & Copy-Move (None) & \num{6.67} & \num{6.58} & \textbf{\num{59.33}} & \textbf{\num{54.96}} & \num{54.01} & \num{53.50} & \num{53.50} & \num{53.13} & \num{18.36} & \num{14.22} \\ \cline{2-12} 
 & Copy-Move (Rotation 180°) & \num{0.04} & \num{0.00} & \num{3.70} & \num{1.42} & \textbf{\num{62.58}} & \textbf{\num{62.24}} & \num{49.83} & \num{49.13} & \num{16.02} & \num{12.89} \\ \cline{2-12} 
 & Copy-Move (Rotation 90°) & \num{0.05} & \num{0.00} & \num{1.66} & \num{0.47} & \num{30.75} & \num{30.55} & \textbf{\num{37.73}} & \textbf{\num{37.15}} & \num{15.07} & \num{12.11} \\ \cline{2-12} 
 & Copy-Move (Retouching) & \num{50.69} & \num{50.49} & \textbf{\num{53.33}} & \textbf{\num{50.49}} & \num{39.10} & \num{38.89} & \num{31.39} & \num{30.79} & \num{16.38} & \num{12.87} \\ \cline{2-12} 
 & Splicing & \num{1.42} & \num{1.33} & \textbf{\num{2.09}} & \num{1.66} & \num{1.99} & \textbf{\num{1.79}} & \num{0.69} & \num{0.49} & \num{1.30} & \num{1.08} \\ \cline{2-12} 
 & Overlap & \num{0.00 }& \num{0.00 }& \num{0.35 }& \num{0.12 }& \num{3.22 }& \num{2.95 }& \textbf{\num{5.86}} & \textbf{\num{5.33}} & \num{8.15 }& \num{5.57 }\\ \cline{2-12} 
 & \textbf{Average} & \num{7.50} & \num{7.41} & \num{16.06} & \num{14.29} & \textbf{\num{24.48}} & \textbf{\num{24.12}} & \num{22.79} & \num{22.25} & \num{13.28} & \num{10.41} \\ \hline  \hline
\multirow{6}{*}{\begin{tabular}[c]{@{}c@{}}Intra-Panel\\ Forgery\end{tabular}} & Cleaning with Brute-Force & \num{0.03} & \num{0.00} & \num{0.21} & \num{0.06} & \num{0.06} & \num{0.02} & \num{0.08} & \num{0.03} & \textbf{\num{1.30}} & \textbf{\num{1.07}} \\ \cline{2-12} 
 & Copy-Move (Flip) & \num{0.00} & \num{0.00} & \num{0.10} & \num{0.04} & \num{0.05} & \num{0.01} & \num{0.06} & \num{0.02} & \textbf{\num{1.30}} & \textbf{\num{1.04}} \\ \cline{2-12} 
 & Copy-Move (Random) & \num{2.26} & \num{2.17} & \textbf{\num{2.38}} & \textbf{\num{1.84}} & \num{2.25} & \num{2.07} & \num{1.40} & \num{1.28} & \num{1.45} & \num{1.19} \\ \cline{2-12} 
 & \textbf{Copy-Move (Rotation)} & \num{0.00} & \num{0.00} & \num{0.11} & \num{0.03} & \num{0.21} & \num{0.14} & \num{0.29} & \num{0.15} & \textbf{\num{1.16}} & \textbf{\num{0.91}} \\ \cline{2-12} 
 & Copy-move (Translation) & \num{0.66} & \num{0.62} & \textbf{\num{1.20}} & \textbf{\num{0.81}} & \num{0.72} & \num{0.52} & \num{0.32} & \num{0.23} & \num{0.80} & \num{0.67} \\ \cline{2-12} 
 & \textbf{Average} & \num{0.59} & \num{0.56} & \num{0.80} & \num{0.55} & \num{0.66} & \num{0.55} & \num{0.43} & \num{0.34} & \textbf{\num{1.20}} & \textbf{\num{0.97}} \\ \hline
\end{tabular}%
\label{tab:compund-f1-l2}
}
\end{table*}

% Please add the following required packages to your document preamble:
% \usepackage{multirow}
% \usepackage{graphicx}
\begin{table*}[]
\caption{Evaluation of Compound Figure Detection on Level 3 of Verbosity with F1-Score}
\resizebox{\textwidth}{!}{%
\begin{tabular}{|c|c|c|c|c|c|c|c|c|c|c|c|}
\hline
\multicolumn{2}{|c|}{\multirow{3}{*}{\textbf{Modality}}} & \multicolumn{10}{c|}{\textbf{Methods (F1-Score - Verbosity Level 3)}} \\ \cline{3-12} 
\multicolumn{2}{|c|}{} & \multicolumn{2}{c|}{ZERNIKE-PM} & \multicolumn{2}{c|}{SIFT-PM} & \multicolumn{2}{c|}{SURF-VOLE} & \multicolumn{2}{c|}{SIFT-VOLE} & \multicolumn{2}{c|}{BUSTERNET} \\ \cline{3-12} 
\multicolumn{2}{|c|}{} &  TP  &  CTP  &  TP  &  CTP  &  TP  &  CTP  &  TP  &  CTP  &  TP  &  CTP  \\ \hline
\multirow{9}{*}{\begin{tabular}[c]{@{}c@{}}Inter-Panel\\ Forgery\end{tabular}} & Copy-Move (Flip) & \num{0.14} & \num{0.03} & \num{6.40} & \num{4.64} & \num{3.01} & \num{2.58} & \num{1.82} & \num{1.46} & \textbf{\num{17.29}} & \textbf{\num{13.17}} \\ \cline{2-12} 
 & Copy-Move (Flip + Rotation 90°) & \num{0.83} & \num{0.83} & \num{1.95} & \num{0.61} & \num{0.72} & \num{0.38} & \num{1.12} & \num{0.61} & \textbf{\num{13.66}} & \textbf{\num{11.34}} \\ \cline{2-12} 
 & Copy-Move (None) & \num{6.75} & \num{6.65} & \textbf{\num{58.85}} & \textbf{\num{54.45}} & \num{52.87} & \num{52.43} & \num{52.75} & \num{52.09} & \num{18.36} & \num{14.21} \\ \cline{2-12} 
 & Copy-Move (Rotation 180°) & \num{0.05} & \num{0.00} & \num{3.94} & \num{1.40} & \textbf{\num{61.88}} & \textbf{\num{61.54}} & \num{49.00} & \num{48.54} & \num{16.03} & \num{12.78} \\ \cline{2-12} 
 & Copy-Move (Rotation 90°) & \num{0.09} & \num{0.00} & \num{1.85} & \num{0.43} & \num{31.23} & \num{31.07} & \textbf{\num{36.35}} & \textbf{\num{35.82}} & \num{15.08} & \num{11.85} \\ \cline{2-12} 
 & Copy-Move (Retouching) & \num{51.14} & \textbf{\num{50.80}} & \textbf{\num{52.84}} & \num{48.16} & \num{37.79} & \num{37.56} & \num{30.45} & \num{29.63} & \num{16.38} & \num{12.39} \\ \cline{2-12} 
 & Splicing & \num{1.68} & \num{1.55} & \num{1.98} & \num{1.50} & \textbf{\num{2.05}} & \textbf{\num{1.90}} & \num{0.71} & \num{0.48} & \num{1.29} & \num{1.06} \\ \cline{2-12} 
 & Overlap & \num{0.00} & \num{0.00} & \num{0.37} & \num{0.17} & \num{3.12} & \num{2.99} & \num{5.68} & \num{5.20} & \textbf{\num{8.15}} & \textbf{\num{5.56}} \\ \cline{2-12} 
 & \textbf{Average} & \num{7.58} & \num{7.48} & \num{16.02} & \num{13.92} & \textbf{\num{24.08}} & \textbf{\num{23.80}} & \num{22.23} & \num{21.73} & \num{13.28} & \num{10.29} \\ \hline \hline
\multirow{6}{*}{\begin{tabular}[c]{@{}c@{}}Intra-Panel\\  Forgery\end{tabular}} & Cleaning (Brute-Force) & \num{0.06} & \num{0.02} & \num{0.27} & \num{0.10} & \num{0.08} & \num{0.03} & \num{0.13} & \num{0.05} & \textbf{\num{1.30}} & \textbf{\num{1.06}} \\ \cline{2-12} 
 & Copy-Move (Flip) & \num{0.00} & \num{0.00} & \num{0.08} & \num{0.02} & \num{0.01} & \num{0.00} & \num{0.02} & \num{0.01} & \textbf{\num{1.30}} & \textbf{\num{1.08}} \\ \cline{2-12} 
 & Copy-Move (Random) & \textbf{\num{2.50}} & \textbf{\num{2.44}} & \num{2.37} & \num{1.69} & \num{2.03} & \num{1.88} & \num{1.39} & \num{1.25} & \num{1.45} & \num{1.18} \\ \cline{2-12} 
 & Copy-Move (Rotation) & \num{0.00} & \num{0.00} & \num{0.09} & \num{0.02} & \num{0.20} & \num{0.13} & \num{0.23} & \num{0.11} & \textbf{\num{1.16}} & \textbf{\num{0.89}} \\ \cline{2-12} 
 & Copy-move (Translation) & \num{0.84} & \num{0.73} & \textbf{\num{1.30}} & \textbf{\num{0.89}} & \num{0.68} & \num{0.52} & \num{0.45} & \num{0.33} & \num{0.80} & \num{0.65} \\ \cline{2-12} 
 & \textbf{Average} & \num{0.68} & \num{0.64} & \num{0.82} & \num{0.54} & \num{0.60} & \num{0.51} & \num{0.44} & \num{0.35} & \textbf{\num{1.20}} & \textbf{\num{0.97}} \\ \hline
\end{tabular}%
\label{tab:compund-f1-l3}
}
\end{table*}

% Please add the following required packages to your document preamble:
% \usepackage{multirow}
% \usepackage{graphicx}
\begin{table*}[]
\caption{Evaluation of Compound Figure Detection on Level 1 of Verbosity with Precision}
\centering
\resizebox{\textwidth}{!}{%
%\begin{tabular}{|c|c|c|c|c|c|c|c|c|c|c|c|}
\begin{tabular}{|c|c|S|S|S|S|S|S|S|S|S|S|}
\hline
\multicolumn{2}{|c|}{\multirow{3}{*}{\textbf{Modality}}} & \multicolumn{10}{c|}{\textbf{Methods (Precision - Verbosity Level 1)}} \\ \cline{3-12} 
\multicolumn{2}{|c|}{} & \multicolumn{2}{c|}{ZERNIKE-PM} & \multicolumn{2}{c|}{SIFT-PM} & \multicolumn{2}{c|}{SURF-VOLE} & \multicolumn{2}{c|}{SIFT-VOLE} & \multicolumn{2}{c|}{BUSTERNET} \\ \cline{3-12} 
\multicolumn{2}{|c|}{} &  TP  &  CTP  &  TP  &  CTP  &  TP  &  CTP  &  TP  &  CTP  &  TP  &  CTP  \\ \hline
\multirow{9}{*}{\begin{tabular}[c]{@{}c@{}}Inter-Panel\\ Forgery\end{tabular}} & Copy-Move (Flip) & \num{1.53} & \num{0.23} & \num{10.15} & \num{7.92} & \num{8.28} & \num{7.24} & \num{8.05} & \num{7.68} & \textbf{\num{10.72}} & \textbf{\num{7.93}} \\ \cline{2-12} 
 & Copy-Move (Flip + Rotation 90°) & \num{1.39} & \num{1.08} & \num{3.94} & \num{1.43} & \num{1.73} & \num{1.52} & \num{3.49} & \num{3.26} & \textbf{\num{8.23}} & \textbf{\num{6.74}} \\ \cline{2-12} 
 & Copy-Move (None) & \num{10.86} & \num{9.99} & \num{50.04} & \num{47.75} & \num{60.41} & \num{59.98} & \textbf{\num{65.12}} & \textbf{\num{65.12}} & \num{11.68} & \num{8.89} \\ \cline{2-12} 
 & Copy-Move (Rotation 180°) & \num{0.65} & \num{0.00} & \num{6.46} & \num{2.49} & \textbf{\num{71.43}} & \textbf{\num{71.01}} & \num{69.89} & \num{69.89} & \num{9.79} & \num{7.88} \\ \cline{2-12} 
 & Copy-Move (Rotation 90°) & \num{0.29} & \num{0.00} & \num{4.12}& \num{0.98} & \num{41.29} & \num{41.14} & \textbf{\num{50.59} }& \textbf{\num{50.59}} & \num{9.17} & \num{7.20}\\ \cline{2-12} 
 & Copy-Move (Retouching) & \textbf{\num{64.22}} & \textbf{\num{63.88}} & \num{48.02} & \num{45.06} & \num{46.42} & \num{46.42} & \num{44.82} & \num{44.82} & \num{9.94} & \num{7.75} \\ \cline{2-12} 
 & Splicing & \num{2.48} & \num{2.38} & \num{1.51} & \num{1.20} & \textbf{\num{2.52}} & \textbf{\num{2.40}} & \num{1.52} & \num{1.48} & \num{0.66} & \num{0.55} \\ \cline{2-12} 
 & Overlap & \num{0.00} & \num{0.00} & \num{0.55} & \num{0.16} & \num{3.67} & \num{3.58} & \textbf{\num{8.20}} & \textbf{\num{7.95}} & \num{4.63} & \num{2.99} \\ \cline{2-12} 
 & \textbf{Average} & \num{10.18} & \num{9.70} & \num{15.60} & \num{13.37} & \num{29.47} & \num{29.16} & \textbf{\num{31.46}} & \textbf{\num{31.35}} & \num{8.10} & \num{6.24} \\ \hline \hline
\multirow{6}{*}{\begin{tabular}[c]{@{}c@{}}Intra-Panel\\ Forgery\end{tabular}} & Cleaning (Brute-Force) & \num{0.07} & \num{0.04} & \num{0.19} & \num{0.05} & \num{0.00} & \num{0.00} & \num{0.00} & \num{0.00} & \textbf{\num{0.67}} & \textbf{\num{0.55}} \\ \cline{2-12} 
 & Copy-Move (Flip) & \num{0.00} & \num{0.00} & \num{0.13} & \num{0.06} & \num{0.01} & \num{0.01} & \num{0.00} & \num{0.00} & \textbf{\num{0.67}} & \textbf{\num{0.54} }\\ \cline{2-12} 
 & Copy-Move (Random) & \textbf{\num{3.95}} & \textbf{\num{3.82}} & 1.84 & \num{1.38} & \num{3.43} & \num{3.31} & \num{2.51} & \num{2.48} & \num{0.74} & \num{0.61} \\ \cline{2-12} 
 & \textbf{Copy-Move (Rotation)} & \num{0.00} & \num{0.00} & \num{0.05} & \num{0.02} & \num{0.20} & \num{0.17} & \num{0.09} & \num{0.07} & \textbf{\num{0.60}} & \textbf{\num{0.47}} \\ \cline{2-12} 
 & Copy-move (Translation) & \textbf{\num{1.46}} & \textbf{\num{1.39}} & \num{0.91} & \num{0.61} & \num{1.17} & \num{0.99} & \num{0.38} & \num{0.36} & \num{0.41} & \num{0.34} \\ \cline{2-12} 
 & \textbf{Average} & \textbf{\num{1.10}} & \textbf{\num{1.05}} & \num{0.63} & \num{0.42} & \num{0.96} & \num{0.89} & \num{0.60} & \num{0.58} & \num{0.62} & \num{0.50} \\ \hline
\end{tabular}%
\label{tab:compund-p-l1}
}
\end{table*}

% Please add the following required packages to your document preamble:
% \usepackage{multirow}
% \usepackage{graphicx}
\begin{table*}[]
\caption{Evaluation of Compound Figure Detection on Level 2 of Verbosity with Precision}
\centering
\resizebox{\textwidth}{!}{%
%\begin{tabular}{|c|c|c|c|c|c|c|c|c|c|c|c|}
\begin{tabular}{|c|c|S|S|S|S|S|S|S|S|S|S|}
\hline
\multicolumn{2}{|c|}{\multirow{3}{*}{\textbf{Modality}}} & \multicolumn{10}{c|}{\textbf{Methods (Precision - Verbosity Level 2)}} \\ \cline{3-12} 
\multicolumn{2}{|c|}{} & \multicolumn{2}{c|}{ZERNIKE-PM} & \multicolumn{2}{c|}{SIFT-PM} & \multicolumn{2}{c|}{SURF-VOLE} & \multicolumn{2}{c|}{SIFT-VOLE} & \multicolumn{2}{c|}{BUSTERNET} \\ \cline{3-12} 
\multicolumn{2}{|c|}{} & TP  & CTP  & TP  & CTP  & TP  & CTP  & TP  & CTP  & TP  & CTP  \\ \hline
\multirow{9}{*}{\begin{tabular}[c]{@{}c@{}}Inter - Panel\\ Forgery\end{tabular}} & Copy-Move (Flip) & \num{1.28} & \num{0.08} & \num{9.98} & \num{7.70} & \num{7.48} & \num{5.76} & \num{5.28} & \num{3.31} & \textbf{\num{10.71}} & \textbf{\num{8.07}} \\ \cline{2-12} 
 & Copy-Move (Flip + Rotation 90°) & \num{1.61} & \num{1.36} & \num{4.26} & \num{1.30} & \num{2.29} & \num{1.45} & \num{3.72} & \num{1.47} & \textbf{\num{8.21}} & \textbf{\num{6.56}} \\ \cline{2-12} 
 & Copy-Move (None) & \num{11.46} & \num{10.74} & \num{51.41} & \num{47.79} & \num{57.05} & \num{56.34} & \textbf{\num{59.57}} & \textbf{\num{58.90}} & \num{11.66} & \num{8.87} \\ \cline{2-12} 
 & Copy-Move (Rotation 180°) & \num{0.34} & \num{0.00} & \num{6.56} & \num{3.00} & \textbf{\num{67.37}} & \textbf{\num{66.83}} & \num{59.71} & \num{58.59} & \num{9.79} & \num{7.76} \\ \cline{2-12} 
 & Copy-Move ( Rotation 90°) & \num{0.62} & \num{0.00} & \num{3.97} & \num{1.26} & \num{38.19} & \num{37.80} & \textbf{\num{46.67}} & \textbf{\num{45.58}} & \num{9.15} & \num{7.06} \\ \cline{2-12} 
 & Copy-Move (Retouching) & \textbf{\num{64.15}} & \textbf{\num{63.87}} & \num{48.94} & \num{46.11} & \num{45.87} & \num{45.47} & \num{39.24} & \num{37.86} & \num{9.92} & \num{7.63} \\ \cline{2-12} 
 & Splicing & \num{2.22} & \num{2.16} & \num{1.63} & \num{1.30} & \textbf{\num{2.24}} & \textbf{\num{2.08}} & \num{1.51} & \num{1.35} & \num{0.66} & \num{0.55} \\ \cline{2-12} 
 & Overlap & \num{0.00} & \num{0.00} & \num{0.60} & \num{0.11} & \num{3.86} & \num{3.57} & \textbf{\num{6.92}} & \textbf{\num{6.18}} & \num{4.63} & \num{3.08} \\ \cline{2-12} 
 & \textbf{Average} & \num{10.21} & \num{9.78} & \num{15.92} & \num{13.57} & \textbf{\num{28.04}} & \textbf{\num{27.41}} & \num{27.83} & \num{26.66} & \num{8.09} & \num{6.20} \\ \hline \hline
\multirow{6}{*}{\begin{tabular}[c]{@{}c@{}}Intra-Panel\\ Forgery\end{tabular}} & Cleaning (Brute-Force) & \num{0.23} & \num{0.03} & \num{0.16} & \num{0.04} & \num{0.04} & \num{0.01} & \num{0.07} & \num{0.02} & \textbf{\num{0.67}} & \textbf{\num{0.55}} \\ \cline{2-12} 
 & Copy-Move (Flip) & \num{0.00} & \num{0.00} & \num{0.07} & \num{0.03} & \num{0.03} & \num{0.01} & \num{0.05} & \num{0.01} & \textbf{\num{0.66}} & \textbf{\num{0.53}} \\ \cline{2-12} 
 & Copy-Move (Random) & \textbf{\num{3.40}} & \textbf{\num{3.32}} & \num{1.77} & \num{1.35} & \num{2.87} & \num{2.72} & \num{2.69} & \num{2.59} & \num{0.74} & \num{0.61} \\ \cline{2-12} 
 & \textbf{Copy-Move (Rotation)} & \num{0.00} & \num{0.00} & \num{0.09} & \num{0.03} & \num{0.22} & \num{0.17} & \num{0.35} & \num{0.21} & \textbf{\num{0.59}} & \textbf{\num{0.46}} \\ \cline{2-12} 
 & Copy-move (Translation) & \textbf{\num{1.09}} & \textbf{\num{1.05}} & \num{0.94} & \num{0.63} & \num{1.18} & \num{0.98} & \num{0.44} & \num{0.35} & \num{0.41} & \num{0.34} \\ \cline{2-12} 
 & \textbf{Average} & \textbf{\num{0.94}} & \textbf{\num{0.88}} & \num{0.60} & \num{0.41} & \num{0.87} & \num{0.78} & \num{0.72} & \num{0.64} & \num{0.61} & \num{0.50} \\ \hline
\end{tabular}%
\label{tab:compund-p-l2}
}
\end{table*}

% Please add the following required packages to your document preamble:
% \usepackage{multirow}
% \usepackage{graphicx}
\begin{table*}[]
\caption{Evaluation of Compound Figure Detection on Level 3 of Verbosity with Precision}
\resizebox{\textwidth}{!}{%
\begin{tabular}{|c|c|c|c|c|c|c|c|c|c|c|c|}
\hline
\multicolumn{2}{|c|}{\multirow{3}{*}{\textbf{Modality}}} & \multicolumn{10}{c|}{\textbf{Methods (Precision - Verbosity Level 3)}} \\ \cline{3-12} 
\multicolumn{2}{|c|}{} & \multicolumn{2}{c|}{ZERNIKE-PM} & \multicolumn{2}{c|}{SIFT-PM} & \multicolumn{2}{c|}{SURF-VOLE} & \multicolumn{2}{c|}{SIFT-VOLE} & \multicolumn{2}{c|}{BUSTERNET} \\ \cline{3-12} 
\multicolumn{2}{|c|}{} & TP  & CTP  & TP  & CTP  & TP  & CTP  & TP  & CTP  & TP  & CTP  \\ \hline
\multirow{9}{*}{\begin{tabular}[c]{@{}c@{}}Inter-Panel\\ Forgery\end{tabular}} & Copy-Move (Flip) & \num{1.37} & \num{0.36} & \num{10.57} & \num{8.13} & \num{7.00} & \num{5.73} & \num{5.83} & \num{4.09} & \textbf{\num{10.71}} & \textbf{\num{7.95}} \\ \cline{2-12} 
 & Copy-Move (Flip + Rotation 90°) & \num{1.17} & \num{1.17} & \num{3.90} & \num{1.21} & \num{2.15} & \num{1.14} & \num{3.11} & \num{1.13} & \textbf{\num{8.21}} & \textbf{\num{6.62}} \\ \cline{2-12} 
 & Copy-Move (None) & \num{11.48} & \num{10.65} & \textbf{\num{50.81}} & \textbf{\num{47.22}} & \num{56.99} & \num{56.23} & \textbf{\num{58.72}} & \textbf{\num{57.84}} & \num{11.66} & \num{8.88} \\ \cline{2-12} 
 & Copy-Move (Rotation 180°) & \num{0.34} & \num{0.00} & \num{7.09} & \num{2.89} & \textbf{\num{66.98}} & \textbf{\num{66.46}} & \num{59.42} & \num{58.57} & \num{9.79} & \num{7.70} \\ \cline{2-12} 
 & Copy-Move (Rotation 90°) & \num{0.82} & \num{0.00} & \num{4.10} & \num{1.00} & \num{39.18} & \num{38.80} & \textbf{\num{46.14}} & \textbf{\num{44.70}} & \num{9.16} & \num{6.91} \\ \cline{2-12} 
 & Copy-Move (Retouching) & \textbf{\num{65.26}} & \textbf{\num{64.58}} & \textbf{\num{48.07}} & \num{43.43} & \num{45.44} & \num{45.00} & \num{38.62} & \num{37.06} & \num{9.92} & \num{7.28} \\ \cline{2-12} 
 & Splicing & \num{2.39} & \num{2.29} & \num{1.48} & \num{1.13} & \textbf{\num{2.49}} & \textbf{\num{2.38}} & \num{1.26} & \num{1.08} & \num{0.66} & \num{0.54} \\ \cline{2-12} 
 & Overlap & \num{0.00} & \num{0.00} & \num{0.05} & \num{0.03} & \num{1.24} & \num{1.23} & \textbf{\num{2.28}} & \textbf{\num{2.17}} & \textbf{\num{0.96}} & \textbf{\num{0.51}} \\ \cline{2-12} 
 & \textbf{Average} & \num{10.35} & \num{9.88} & \num{15.76} & \num{13.13} & \textbf{\num{27.68}} & \textbf{\num{27.12}} & \num{26.92} & \num{25.83} & \num{7.63} & \num{5.80} \\  \hline \hline
\multirow{6}{*}{\begin{tabular}[c]{@{}c@{}}Intra-Panel\\ Forgery\end{tabular}} & Cleaning (Brute-Force) & \num{0.31} & \num{0.13} & \num{0.22} & \num{0.07} & \num{0.06} & \num{0.03} & \num{0.11} & \num{0.05} & \textbf{\num{0.67}} & \textbf{\num{0.55}} \\ \cline{2-12} 
 & Copy-Move (Flip) & \num{0.00} & \num{0.00} & \num{0.05} & \num{0.01} & \num{0.00} & \num{0.00} & \num{0.02} & \num{0.01} & \textbf{\num{0.66}} & \textbf{\num{0.55}} \\ \cline{2-12} 
 & Copy-Move (Random) & \textbf{\num{3.71}} & \textbf{\num{3.66}} & \num{1.70} & \num{1.19} & \num{2.90} & \num{2.76} & \num{2.53} & \num{2.41} & \num{0.74} & \num{0.60} \\ \cline{2-12} 
 & Copy-Move (Rotation) & \num{0.00} & \num{0.00} & \num{0.06} & \num{0.01} & \num{0.23} & \num{0.17} & \num{0.27} & \num{0.13} & \textbf{\num{0.59}} & \textbf{\num{0.45}} \\ \cline{2-12} 
 & Copy-move (Translation) & \num{1.33} & \num{1.25} & \textbf{\num{0.95}} & \textbf{\num{0.66}} & \textbf{\num{0.96}} & \textbf{\num{0.79}} & \num{0.63} & \num{0.53} & \num{0.41} & \num{0.33} \\ \cline{2-12} 
 & \textbf{Average} & \textbf{\num{1.07}} & \textbf{\num{1.01}} & \num{0.60} & \num{0.39} & \num{0.83} & \num{0.75} & \num{0.71} & \num{0.63} & \textbf{\num{0.61}} & \textbf{\num{0.50}} \\ \hline
\end{tabular}%
\label{tab:compund-p-l3}
}
\end{table*}

\begin{figure*}[h]
\centering
 \large{Simple Forgery Output Detection Samples}
 
 \centering
 \vspace{0.3cm}
    \includegraphics[width=\textwidth]{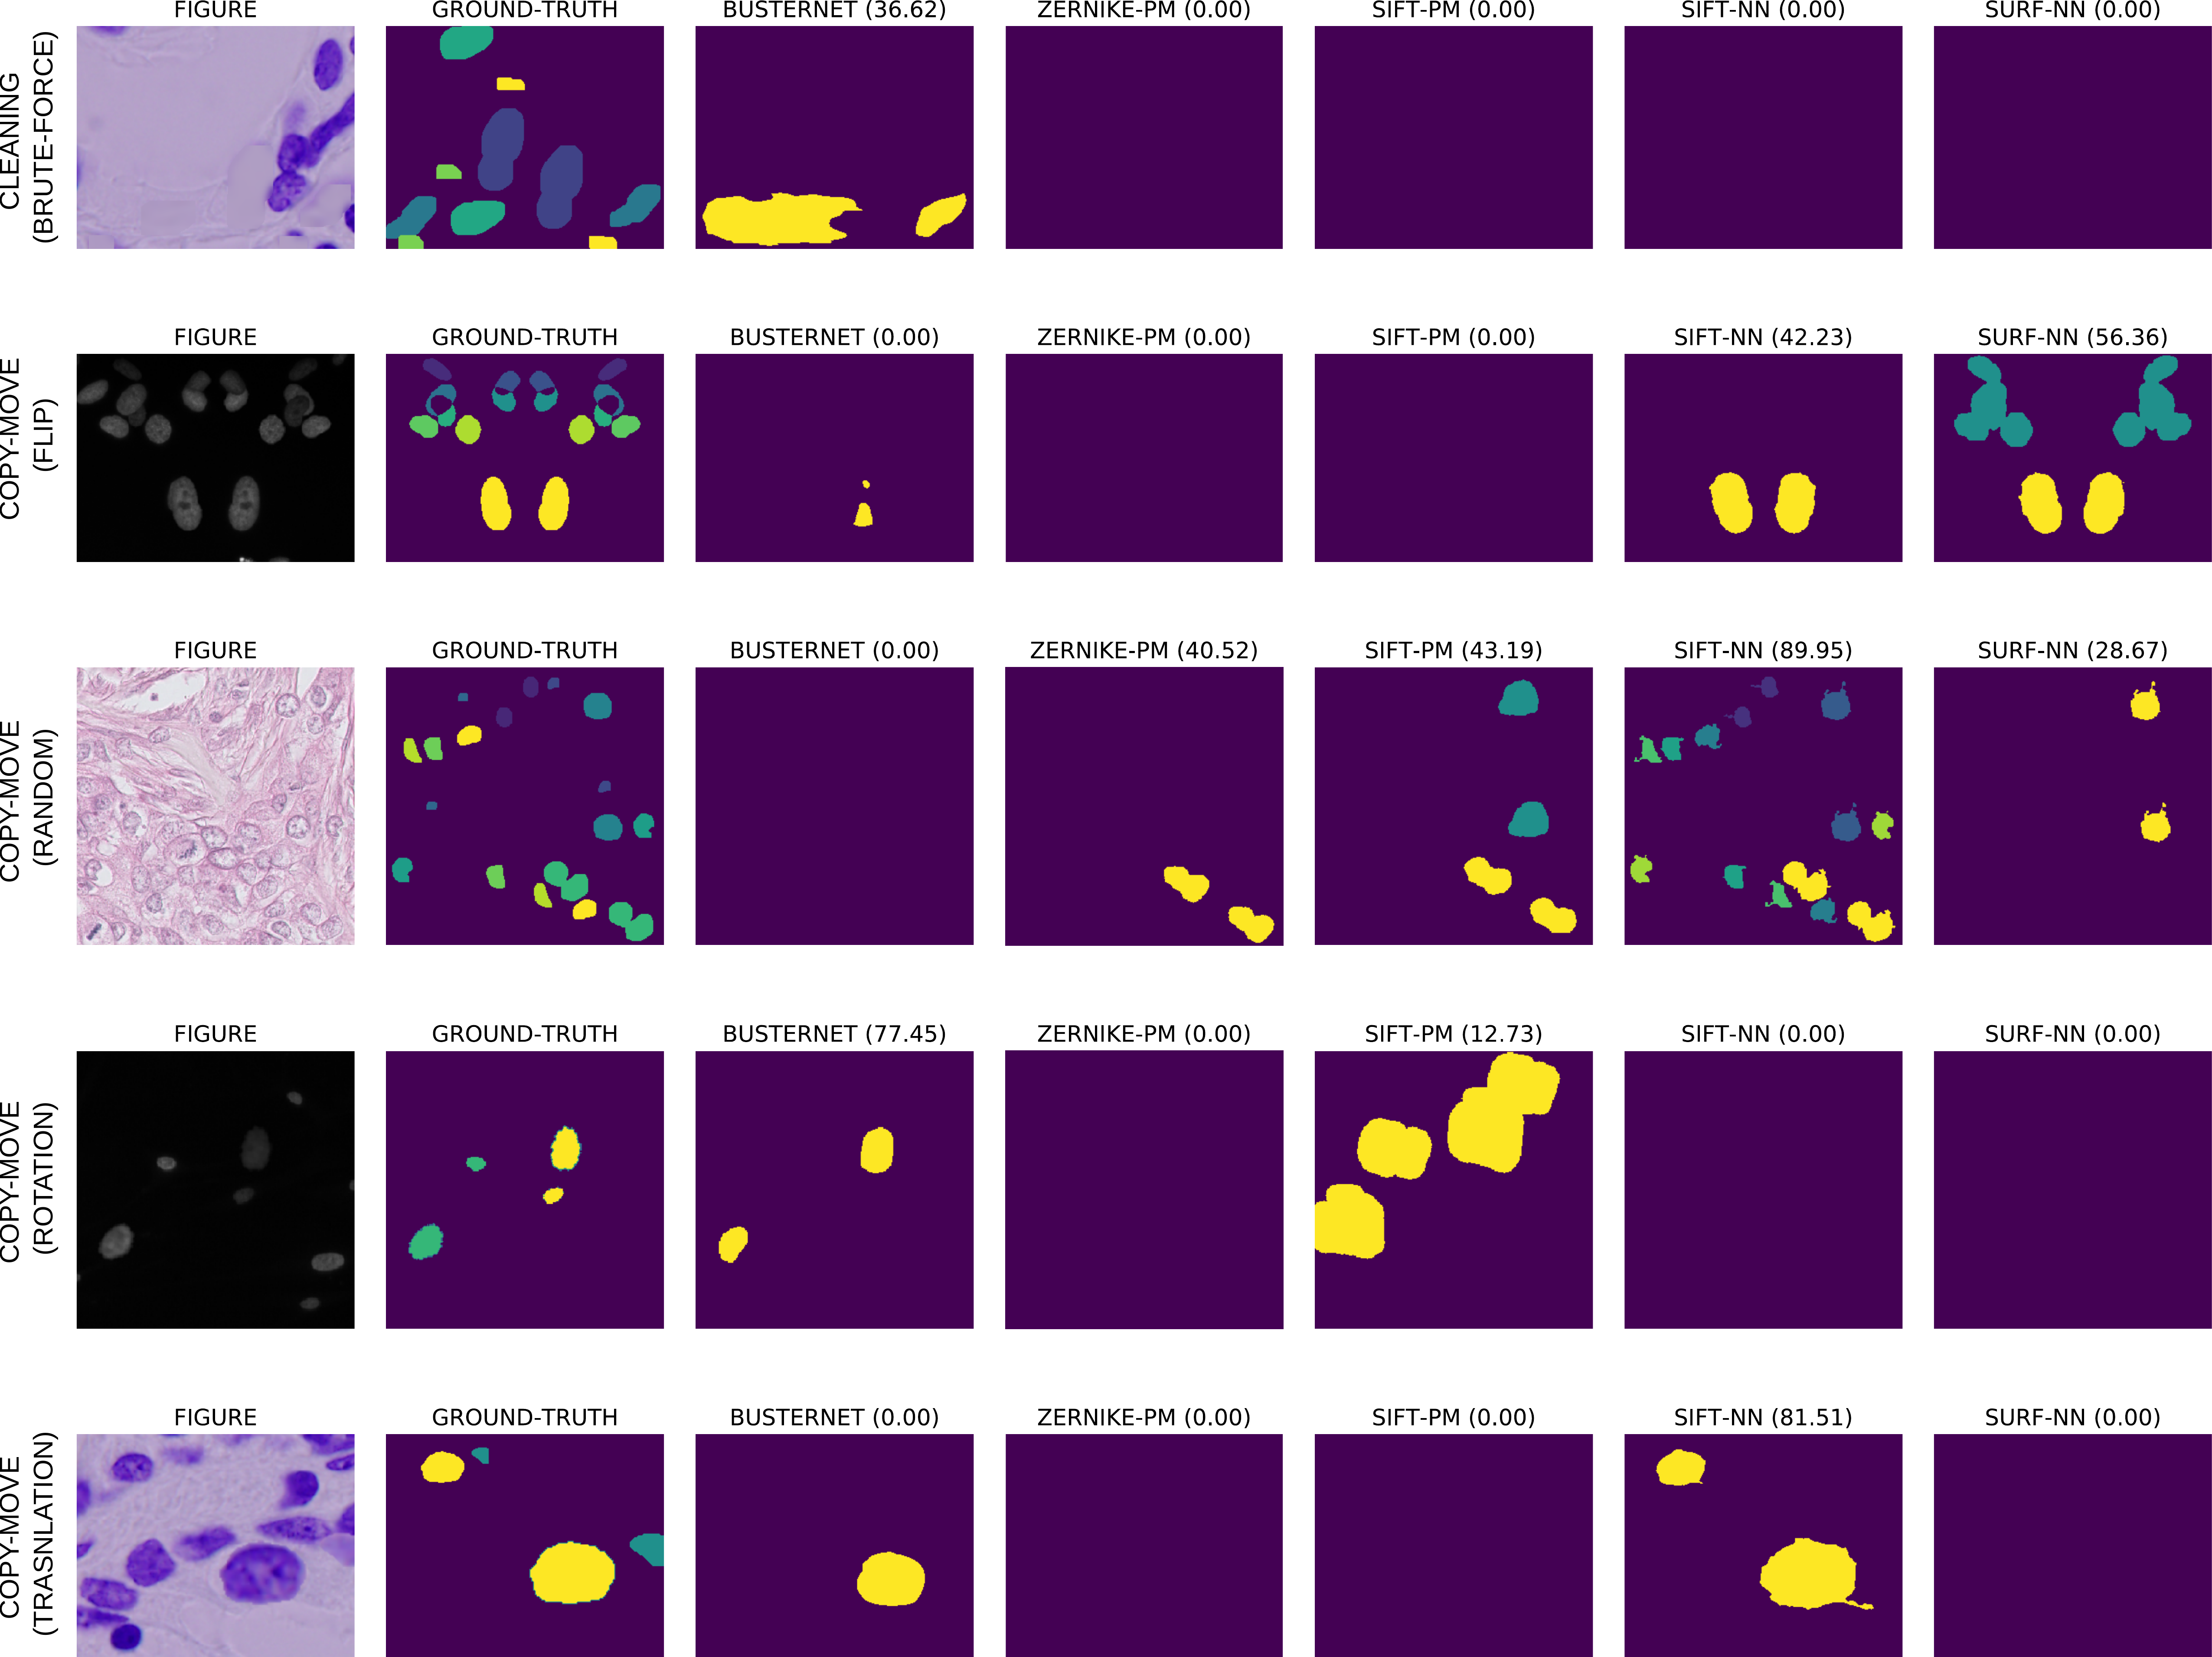}
         \caption{Comparative Simple Forgery duplication detection output per modality. The purple color represents a pristine/non-suspect region, and each other color in the ground-truth and detection maps represents a different ID assigned to each object and its copies. Inside the parenthesis of each method, we insert the $\mbox{F1-score}_{CTP}$ metric normalized into [0, 100].}
\label{fig:sample-simple-forgery}
\end{figure*}

\begin{figure*}
\centering
 \large{Compound Inter-Panel Forgery Output Detection Samples}
 
 \centering
 \vspace{0.3cm}
    \includegraphics[width=\textwidth]{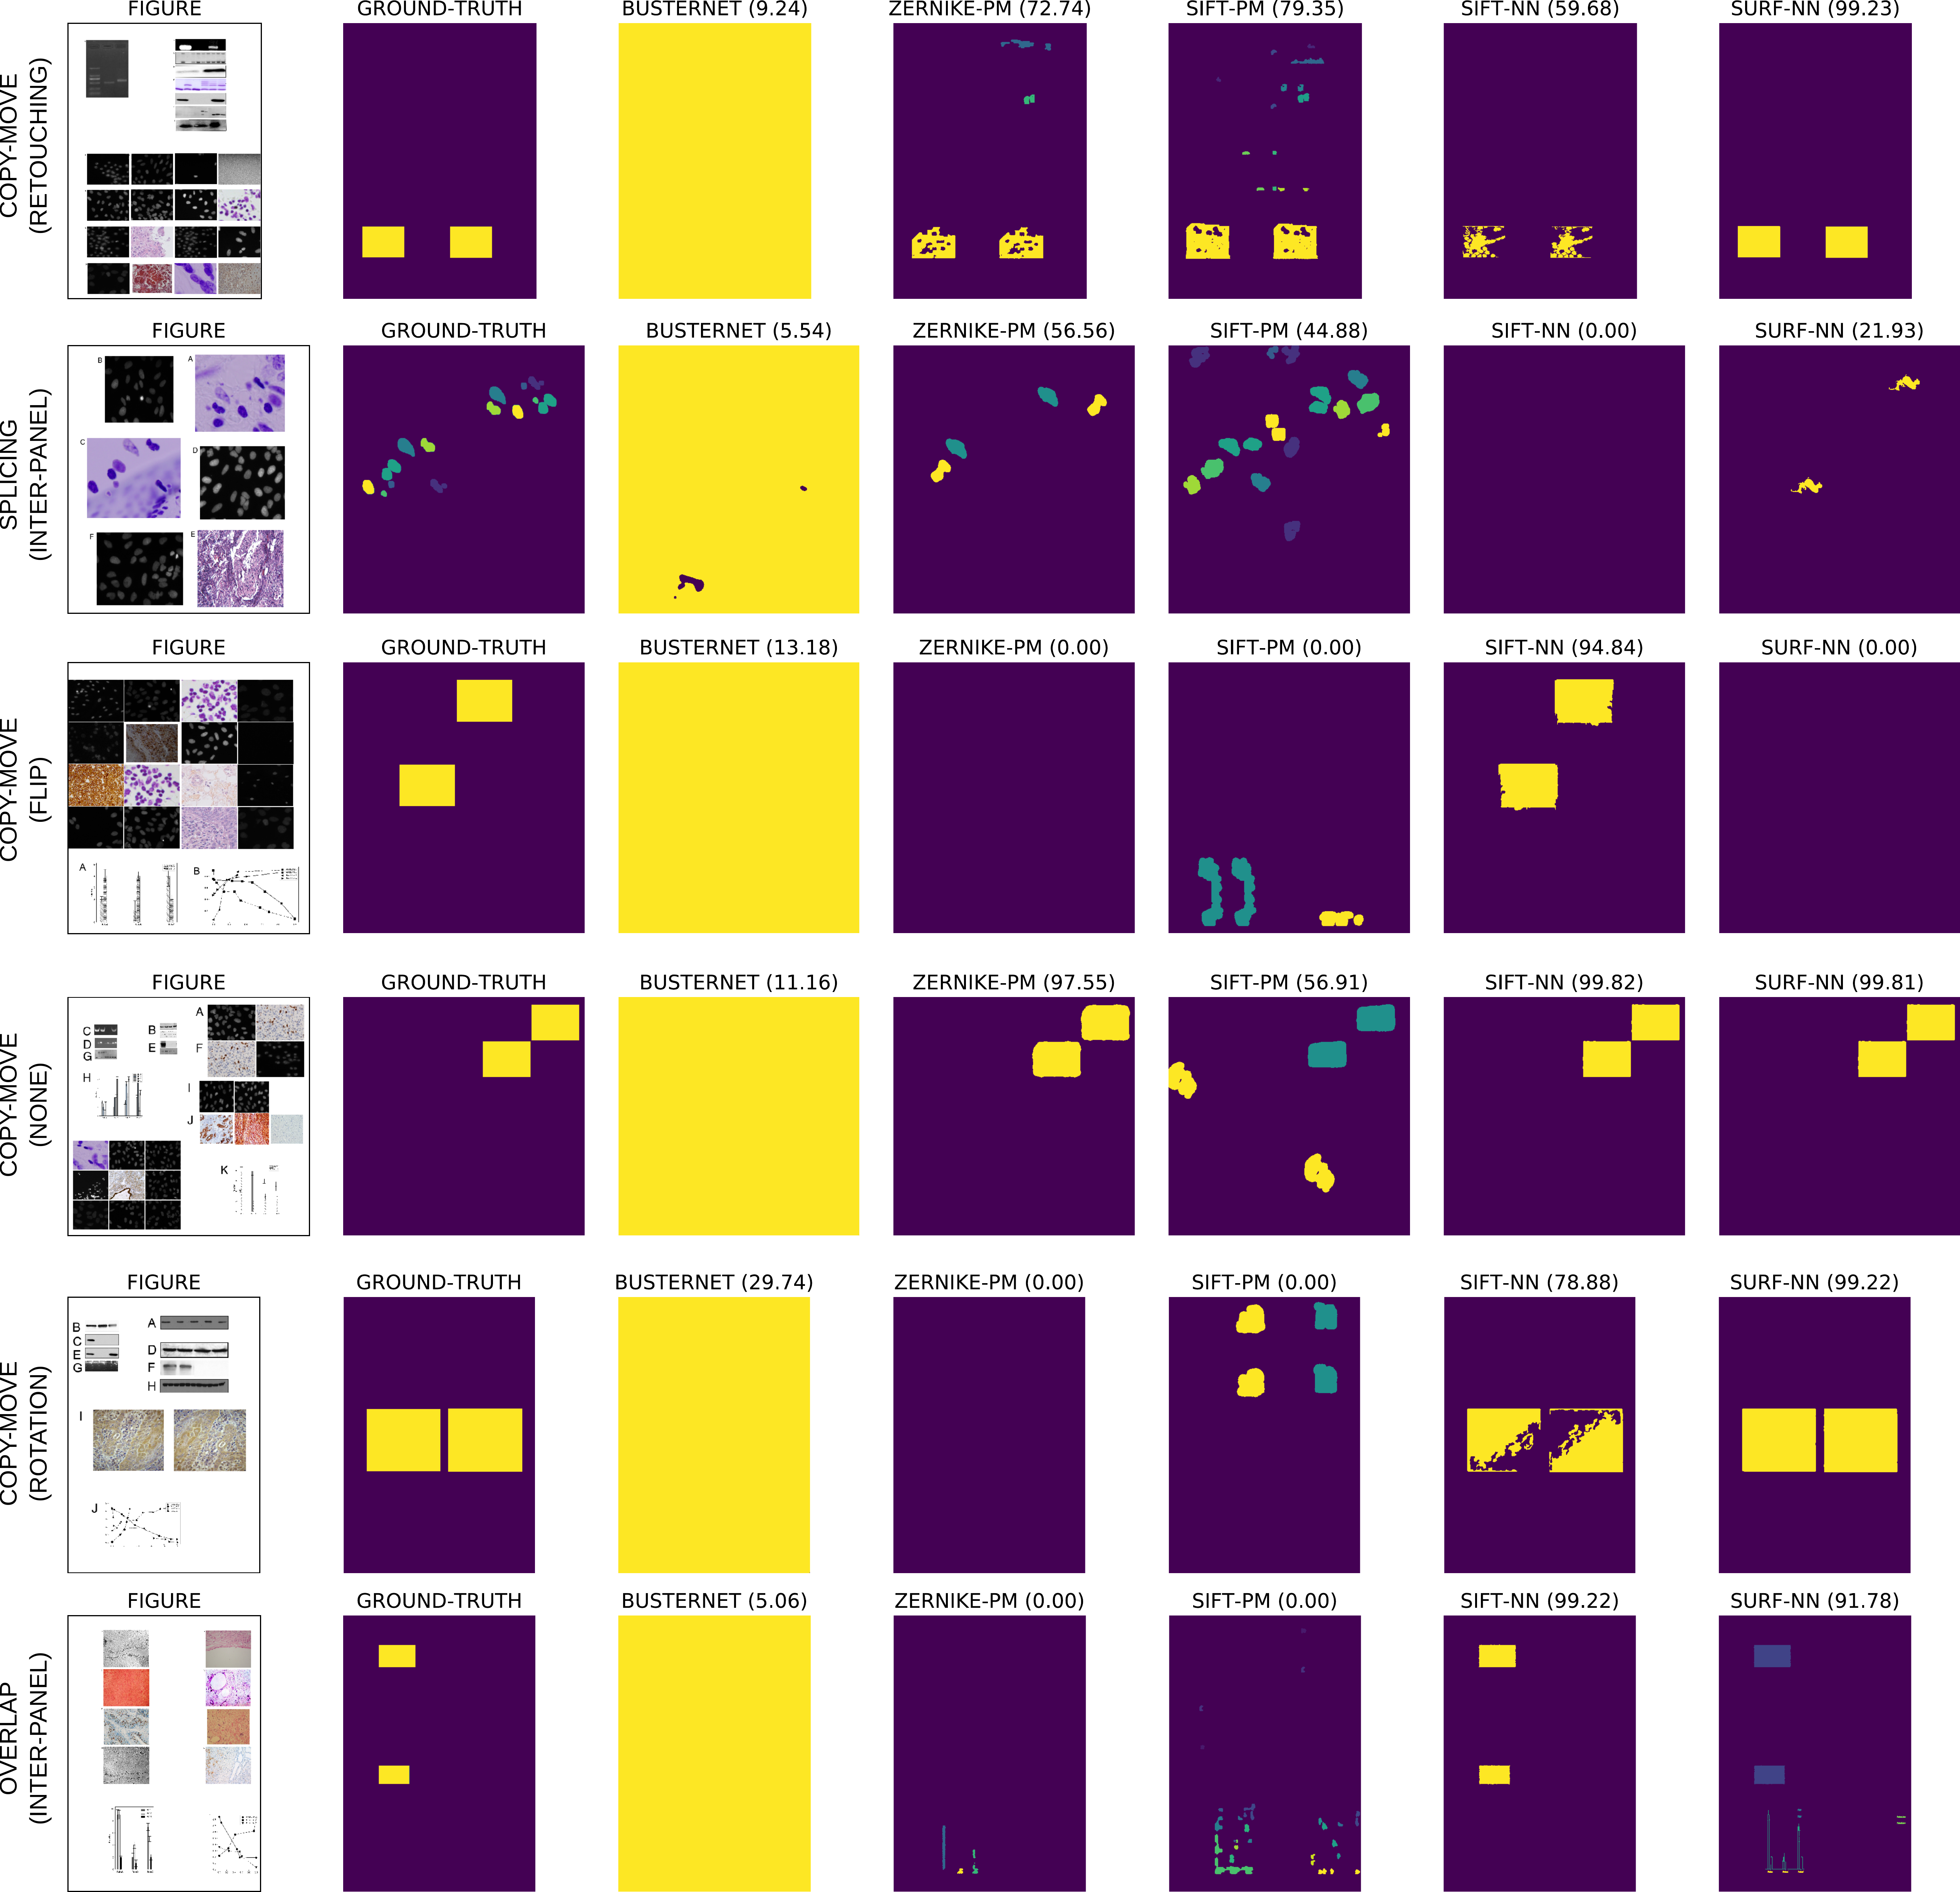}
         \caption{Comparative Compound Inter-Panel Forgery duplication detection output per modality. The purple color represents a pristine/non-suspect region, and each other color in the ground-truth and detection maps represents a different ID assigned to each object and its copies. Inside the parenthesis of each method, we insert the $\mbox{F1-score}_{CTP}$ metric normalized into [0, 100].}
\label{fig:sample-intra-forgery}
\end{figure*}

\begin{figure*}
\centering
 \large{Compound Intra-Panel Forgery Output Detection Samples}
 
 \vspace{0.3cm}
    \includegraphics[width=\textwidth]{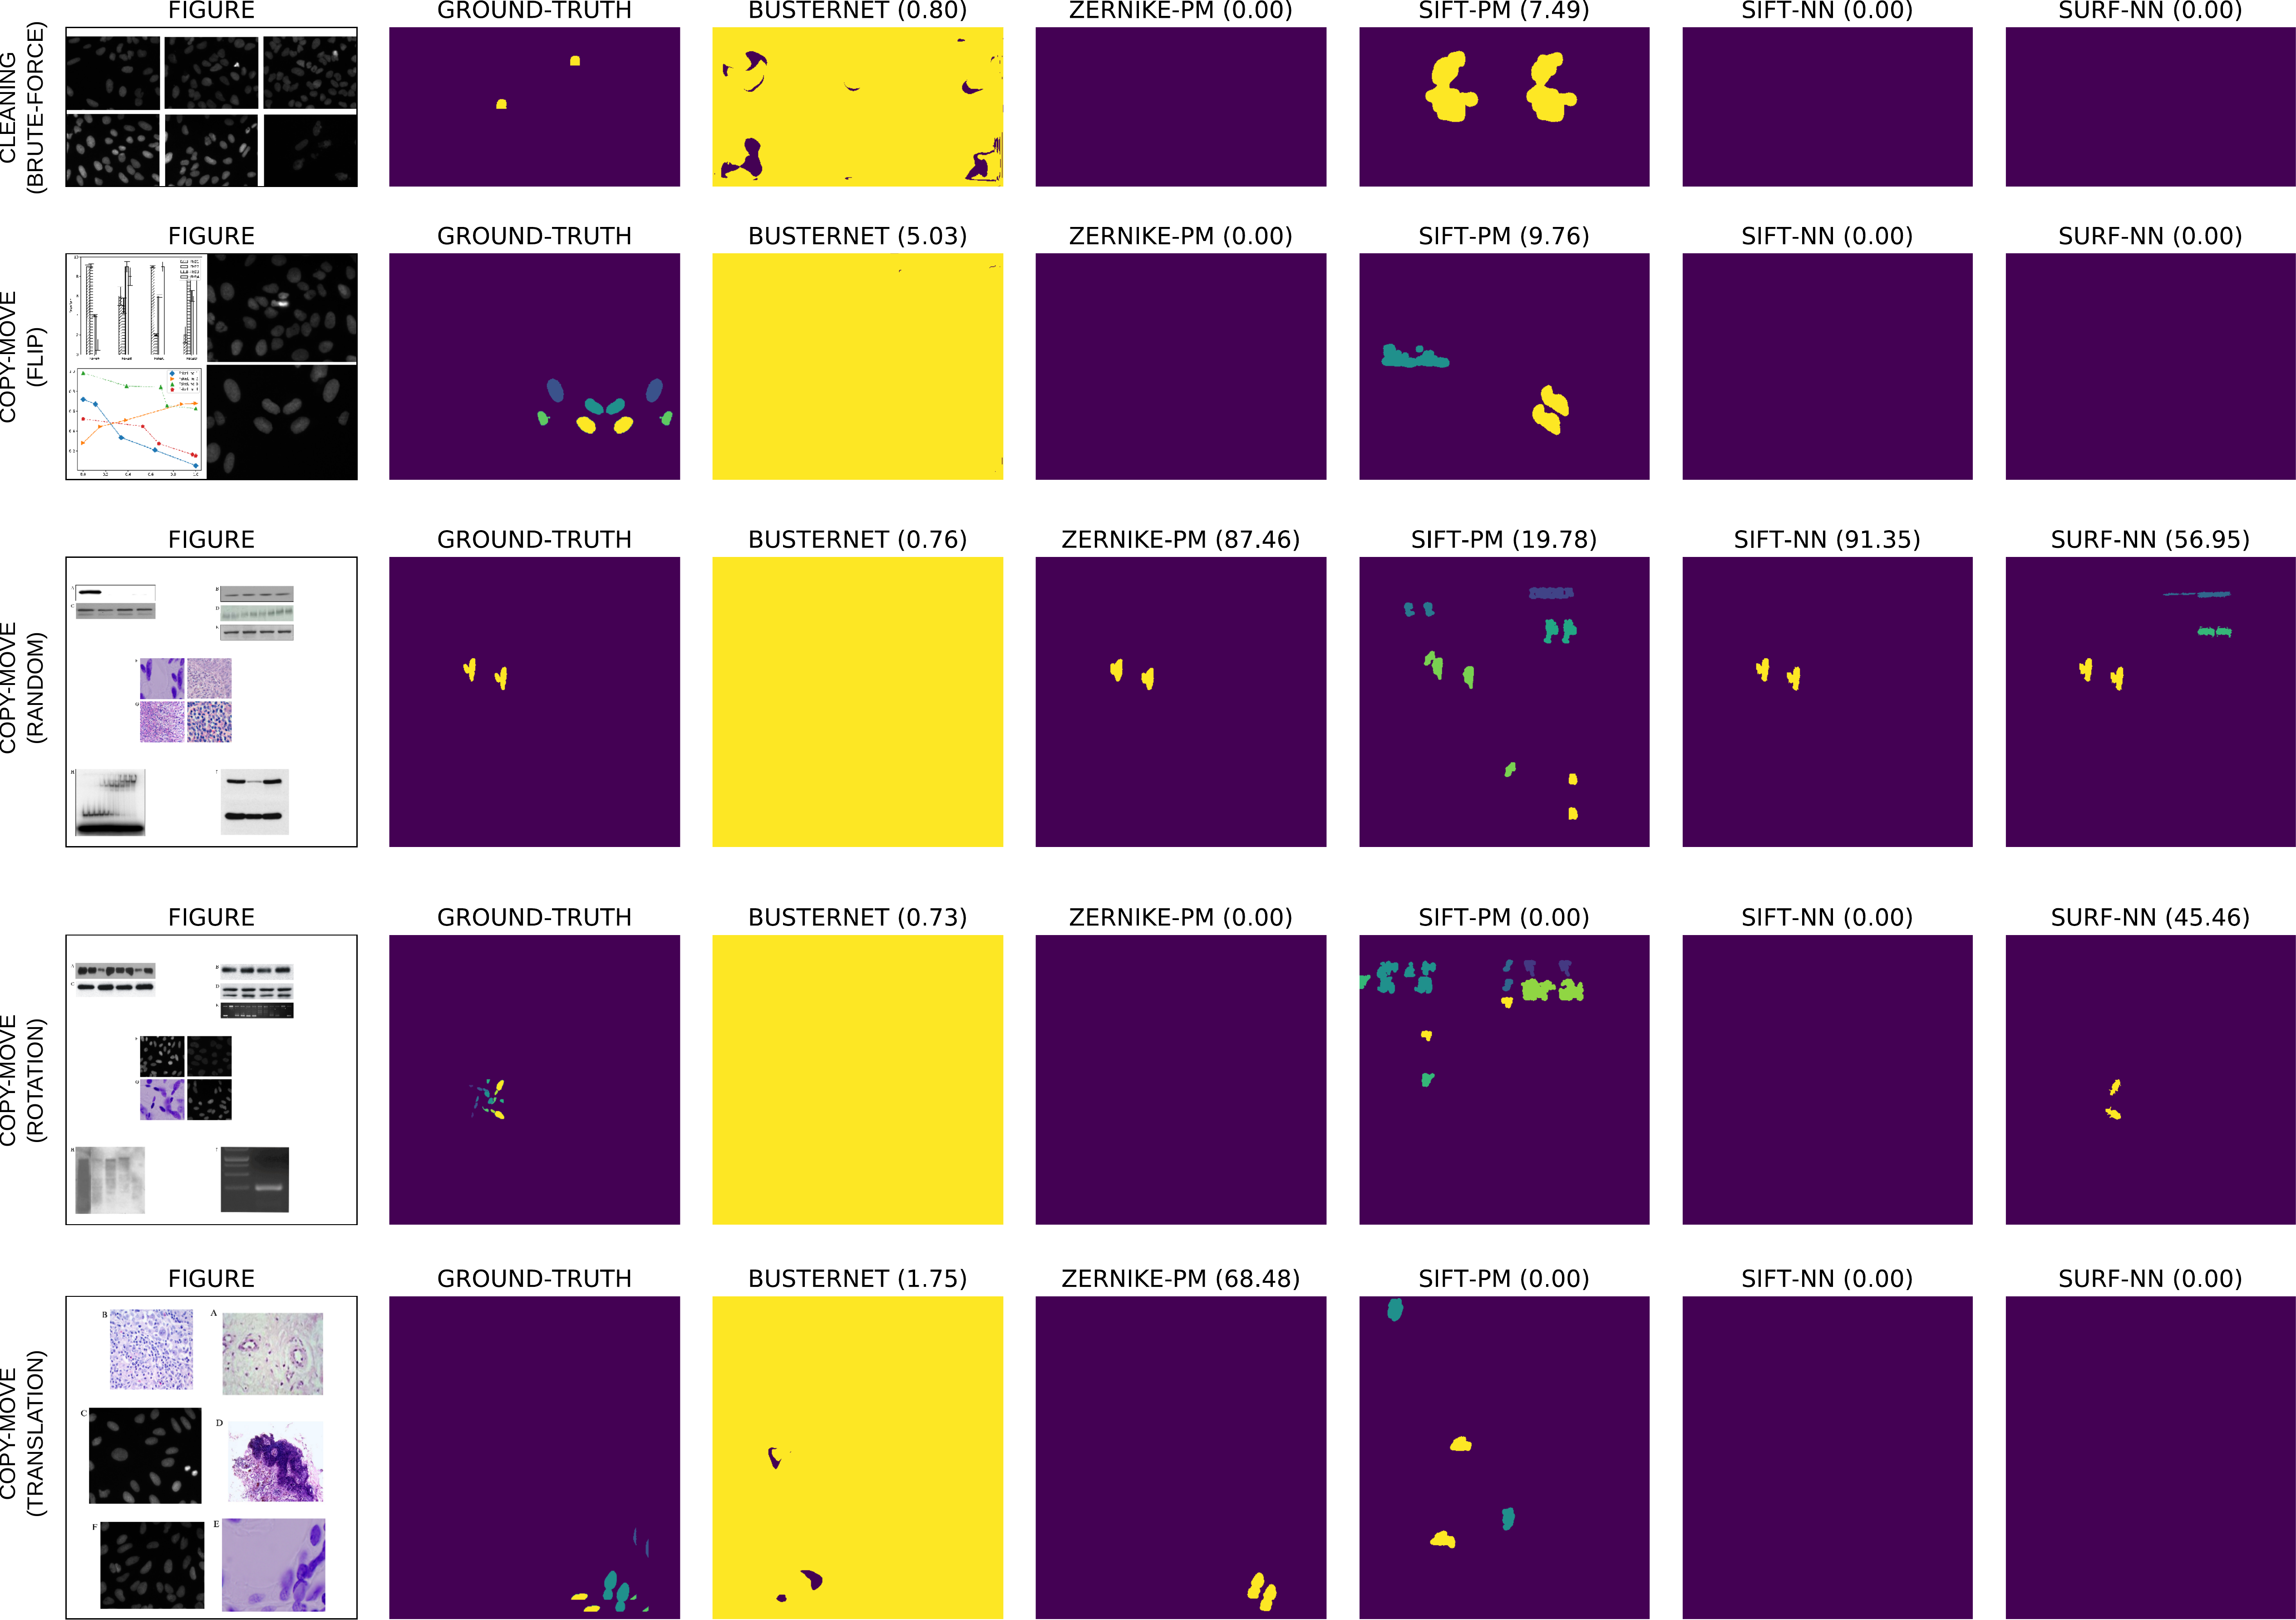}
         \caption{Comparative Compound Intra-Panel Forgery duplication detection output per modality. The purple color represents a pristine/non-suspect region, and each other color in the ground-truth and detection maps represents a different ID assigned to each object and its copies. Inside the parenthesis of each method, we insert the $\mbox{F1-score}_{CTP}$ metric normalized into [0, 100].}
\label{fig:sample-inter-forgery}
\end{figure*}
